# Supplementary material for: Learning interpretable causal networks from very large datasets, application to 400,000 medical records of breast cancer patients
Source: arXiv:2303.06423 ancillary file (2023-03-11)
Supplement: Supplementary file 1 [file ribeiro-dantas_arxiv2023_SI.pdf]

## Supporting Information

# Learning interpretable causal networks from very large datasets, application to 400,000 medical records of breast cancer patients

M.C. Ribeiro-Dantas, H. Li, V. Cabeli, L. Dupuis, F. Simon, L. Hettal, A-S. Hamy, H. Isambert

### 1. Overview and limitations of constraint-based methods

Constraint-based methods (1, 2) proceed through successive steps, outlined in Fig. 1b, whose accuracy ultimately conditions the reliability and interpretability of the final causal graphical model. Starting from a fully connected graph, their first step consists in removing, iteratively, all dispensable edges whenever two variables are marginally independent or conditionally independent given a so-called separating set of conditioning variables. Positive (resp. negative) partial correlations are represented with red (resp. blue) edges in Fig. 1b and all other network figures. The rationale behind this first step is that all statistical associations between disconnected variables in the predicted graph should be graphically interpretable in terms of indirect paths through their separating set. This is, however, frequently not the case in practice (3).

The second step then consists in orienting some of the edges of the undirected graph (named skeleton) obtained at the first step, based on the signature of causality in observational data. This amounts to orient so-called “v-structures” as,  $X \rightarrow Z \leftarrow Y$ , whenever the edge  $X - Y$  has been removed without including a common neighbor  $Z$  of  $X$  and  $Y$  in their separating set,  $\mathcal{S}$ . The converging orientations of such a v-structure graphically indicate that  $Z$  cannot be a cause of neither  $X$  nor  $Y$ , which would otherwise require  $Z$  to be included in the separating set,  $\mathcal{S}$ . However, this does not imply that  $X$  (or  $Y$ ) is an actual cause of  $Z$ , which also requires to rule out the possibility that the direct link between  $X$  and  $Z$  (or  $Y$  and  $Z$ ) might in fact originate from an unmeasured confounder, that is, from a latent common cause,  $L$ , unobserved in the dataset, *i.e.*  $X \leftarrow L \rightarrow Z$ , as described with an intuitive example in Box 1. Finally, the third step aims at propagating the orientations of v-structures to downstream edges, to fulfill the assumptions of the underlying graphical model class of constraint-based methods.

However, while traditional constraint-based methods have been shown to be theoretically sound and complete given an unlimited amount of data (4), they lack robustness on finite datasets, as their long series of uncertain decisions lead to an accumulation of errors, which limit the reliability of the final networks. In particular, spurious conditional independences, stemming from coincidental combinations of conditioning variables, lead to many false negative edges and, ultimately, limit the accuracy of inferred orientations.

### 2. Overview and limitations of MIIC method

The recent causal discovery method, MIIC, combines constraint-based and information-theoretic frameworks to learn more robust causal graphical models (5, 6). To limit the accumulation of errors in removing dispensable edges, MIIC does not directly attempt to uncover conditional independences but, instead, iteratively substracts the most significant information contributions of successive contributors,  $A_1, A_2, \dots, A_n$ , from the mutual information between each pair of variables,  $I(X; Y)$ , as,

$$I(X; Y) - I(X; Y; A_1) - I(X; Y; A_2|A_1) - \dots - I(X; Y; A_n|\{A_i\}_{i=1}^{n-1}) = I(X; Y|\{A_i\}_n) \quad [1]$$

where  $I(X; Y; A_k|\{A_i\}_{i=1}^{k-1}) > 0$  is the *positive* information contribution from  $A_k$  to  $I(X; Y)$ , that is not dependent on the first  $k - 1$  collected variables,  $\{A_i\}_{i=1}^{k-1}$  (7, 8). Conditional independence is eventually established when the residual conditional mutual information on the right hand side of Eq. 1,  $I(X; Y|\{A_i\}_n)$ , becomes smaller than a complexity term, *i.e.*  $k_{X; Y|\{A_i\}}(N) \geq I(X; Y|\{A_i\}_n) \geq 0$ , which depends on the considered variables and sample size  $N$ . This complexity term also defines size corrected (or “regularized”) conditional mutual information as,

$$I'(X; Y|\{A_i\}_n) = I(X; Y|\{A_i\}_n) - k_{X; Y|\{A_i\}}(N) \quad [2]$$

which become *negative* under conditional independence (*i.e.*  $I'(X; Y|\{A_i\}_n) \leq 0$ ), that is, whenever sufficient and significant indirect positive contributions could be iteratively collected in Eq. 1 to warrant the removal of edge  $XY$ .

This leads to an undirected skeleton, which MIIC then (partially) orients based on the sign and amplitude of the regularized conditional 3-point information terms (5, 7), corresponding to the difference between regularized conditional mutual information terms.

$$I'(X; Y; Z|\{A_i\}) = I'(X; Y|\{A_i\}) - I'(X; Y|\{A_i\}, Z) \quad [3]$$

In particular, negative conditional 3-point information terms,  $I'(X; Y; Z|\{A_i\}) < 0$ , correspond to the signature of causality in observational data (7) and lead to the prediction of a v-structure,  $X \rightarrow Z \leftarrow Y$ , if  $X$  and  $Y$  are not connected in the skeleton (with  $I'(X; Y|\{A_i\}) \leq 0$ ). By contrast, a positive conditional 3-point information term,  $I'(X; Y; Z|\{A_i\}) > 0$ , implies the absence of a v-structure and suggests to propagate the orientation of a previously directed edge  $X \rightarrow Z - Y$  as  $X \rightarrow Z \rightarrow Y$  (with  $I'(X; Y|\{A_i\}, Z) \leq 0$ ), to fulfill the assumptions of the underlying graphical model class.

In practice, MIIC’s strategy to circumvent spurious conditional independences significantly improves the sensitivity or recall, that is, the fraction of correctly recovered edges, compared to traditional constraint-based methods, Fig. S3. However, original MIIC as well as all other causal discovery methods still present a number of major limitations, such as (i) a lower

reliability in predicting edge orientation than edge presence, (ii) a poor scalability, notably with continuous or mixed-type data, (iii) a remaining ambiguity on the “putative” *versus* “genuine” causal nature of oriented edges (Box 1), and (iv) a frequent inconsistency of separating sets with respect to indirect paths in the inferred network. The advanced iMIIC method overcomes all these limitations, as detailed in the following sections.

### 3. Improved reliability of iMIIC inferred orientations

While the original MIIC significantly outperforms traditional constraint-based methods in inferring reliable orientations, a substantial loss in precision usually remains between MIIC skeleton and oriented graph predictions, Fig. S3. This is due to orientation errors originating from inconsistent v-structures,  $X \rightarrow Z \leftarrow Y$ , whose middle node  $Z$  could also be included in the separating set of the unconnected pair  $\{X, Y\}$ , in contradiction with the head-to-head meeting of the v-structure. In particular, for discrete variables with (too) many levels, complexity terms can easily outweigh (conditional) mutual information for weakly dependent variables. As a result, original MIIC tends to infer some v-structure orientations,  $X \rightarrow Z \leftarrow Y$ , for which both (conditional) mutual information terms in Eq. 3 are negative, *i.e.*  $I'(X; Y|\{A_i\}) < I'(X; Y|\{A_i\}, Z) < 0$ , suggesting that  $Z$  could in fact be included in a separating set of the  $\{X, Y\}$  pair, in contradiction with the inferred v-structure,  $X \rightarrow Z \leftarrow Y$ . To circumvent this issue, iMIIC implements more conservative orientation rules by essentially treating categorical and continuous variables alike, based on a general mutual information supremum principle (9, 10), outlined below. In particular, Theorem 1, below, requires to rectify all negative regularized (conditional) mutual information, defining (conditional) independence (*e.g.*  $I'(X; Y|\{A_i\}) \leq I'(X; Y|\{A_i\}, Z) \leq 0$ ), to null values (*i.e.*  $I'(X; Y|\{A_i\}) = I'(X; Y|\{A_i\}, Z) = 0$ ), which leads to vanishing conditional 2-point and 3-point information in Eq. 3, for the example above, and prevents the orientation of all inconsistent v-structures.

**General mutual information supremum principle.** Estimating (conditional) mutual information between continuous or mixed-type variables is notoriously more challenging than between categorical variables (11, 12). Original MIIC computes regularized mutual information between continuous or mixed-type variables through an optimum discretization scheme, based on a general mutual information supremum principle (9) regularized for finite datasets and using an efficient  $\mathcal{O}(N^2)$  dynamic programming algorithm (6). This approach finds optimum partitions,  $\mathcal{P}$  and  $\mathcal{Q}$ , specifying the number and positions of cut-points of each continuous variable,  $X$  and  $Y$ , to maximize the regularized mutual information between them,

$$I'(X; Y) = \sup_{\mathcal{P}, \mathcal{Q}} I'([X]_{\mathcal{P}}; [Y]_{\mathcal{Q}}) \quad [4]$$

Such optimization-based estimates of mutual information are at par with alternative distance-based k-nearest neighbor (kNN) approaches (11, 12) but have also the unique advantage of providing an effective independence test to identify independent continuous or mixed-type variables (6). This is achieved when partitioning  $X$  and  $Y$  into single bins maximizes the regularized mutual information in Eq. 4, which vanishes exactly in this case, *i.e.*  $I'(X; Y) = I'([X]_1; [Y]_1) = 0$  if  $I'([X]_{\mathcal{P}}; [Y]_{\mathcal{Q}}) \leq 0$  for all partitions  $\mathcal{P}, \mathcal{Q}$ . By contrast, kNN estimates still need an actual independence test to decide whether some variables are effectively independent or not, as kNN mutual information estimates are never exactly null.

Yet, the optimum partitioning principle (Eq. 4) only applies to mutual information (9), *not* conditional mutual information, which need to be estimated through the *difference* between optimum regularized mutual information terms, as  $I'(X; Y|U) = I'(Y; \{X, U\}) - I'(Y; U) = I'(X; \{Y, U\}) - I'(X; U)$  (6). As a result of numerical approximation, the regularized conditional mutual information estimates between conditionally independent variables can sometime be negative and lead to inconsistent v-structure orientations, as discussed for discrete data above.

The general mutual information supremum principle (9), regularized for finite datasets in Eq. 4, is theoretically valid for any type of variable, not just continuous variables. In particular, it could be applied to datasets including discrete or categorical variables with (too) many levels. This would result in the merging of rare levels to better estimate mutual information and conditional mutual information between weakly dependent discrete variables. Ultimately, mutual information estimates between independent discrete variables should lead to the merging of each variable into a single bin, thereby, resulting in regularized mutual information estimates to vanish exactly in this case, as observed for continuous variables. As a result, optimum regularized mutual information should be non-negative as well as, by extension, regularized conditional mutual information, as proved below.

**Theorem 1.** Regularized (conditional) mutual information derived from the general mutual information supremum principle are non-negative.

**Proof.** We first address optimum regularized mutual information without conditioning variables, noting that  $I'(X; Y) \geq I'([X]_1; [Y]_1) = 0$ , where  $[X]_1$  and  $[Y]_1$  are the  $X$  and  $Y$  variables partitioned into single bins, which leads to a vanishing regularized mutual information, as both mutual information and complexity cost are null for single bin partitions (7). Then, regularized conditional mutual information is defined as the *difference* between optimum regularized mutual information terms as,  $I'(X; Y|U) = I'(Y; \{X, U\}) - I'(Y; U) = I'(X; \{Y, U\}) - I'(X; U)$ . However, partitioning  $X$  and  $Y$  into single bins leads to  $I'(Y; \{X, U\}) \geq I'(Y; \{[X]_1, U\}) = I'(Y; U)$  and  $I'(X; \{Y, U\}) \geq I'(X; \{[Y]_1, U\}) = I'(X; U)$  thus implying  $I'(X; Y|U) \geq 0$   $\square$

Hence, Theorem 1 requires to rectify all negative values of regularized (conditional) mutual information, indicating (conditional) independence, to null values instead. Enforcing this rectification of regularized (conditional) mutual information

terms is found to significantly enhance the reliability of iMIIC predicted orientations, in particular for datasets with high proportions of discrete variables, with only a small sensitivity loss compared to MIIC original orientation rules, Fig. 1c.

#### 4. Scalable computations of multivariate information and iMIIC orientation scores

The running time of the original MIIC algorithm scales linearly with sample size for discrete datasets (5) but at best quadratically with sample size for continuous or mixed-type datasets (6), due to a  $\mathcal{O}(N^2)$  dynamic programming optimization of the number and positions of cut points to estimate (conditional) multivariate information. This quadratic scaling becomes prohibitive for very large datasets, such as the SEER dataset analyzed here, which contains nearly 400,000 breast cancer patients. To circumvent this scalability issue, iMIIC enforces a maximum number of 50 bins, so that the overall optimisation of multivariate information estimates remains close to linear in terms of sample size, see Figs. S4-S6. While introducing a maximum number of bins slightly underestimates mutual information between strongly associated variables in very large datasets (*i.e.* when the actual supremum is achieved with more bins in Eq. 4), it has in fact very little effect on iMIIC's results in practice. In particular, the critical first step assessing (conditional) independence between variables (*i.e.* step 1 in Fig. 1b) is achieved by partitioning these variables into single bins, as discussed above, and is therefore completely insensitive to the actual maximum number of bins in the algorithm.

A second scalability issue concerns the estimation of orientation probabilities by the original MIIC, which are numerically too close to be reliably compared for very large datasets and require to introduce scalable orientation scores and novel definitions of induced tail and head orientation scores, as detailed now.

**V-structure orientation scores.** Head orientation probabilities of v-structures,  $X * \rightarrow Z \leftarrow * Y$ , are computed from negative regularized (conditional) 3-point information,  $I'(X; Y; Z | \{A_i\}) < 0$ , as, (5)

$$P(x * \rightarrow z) = P(z \leftarrow * y) = \frac{1 + e^{N I'(X; Y; Z | \{A_i\})}}{1 + 3e^{N I'(X; Y; Z | \{A_i\})}} \geq \frac{1}{2} \quad [5]$$

where the end mark (\*) stands either for a head (>), a tail (-) or is undefined (o), and  $e^{N I'(X; Y; Z | \{A_i\})}$  corresponds to the probability ratio between a non-v-structure and a v-structure,  $e^{N I'(X; Y; Z | \{A_i\})} = P_{\rightarrow -} / P_{\rightarrow \leftarrow} = P_{\leftarrow -} / P_{\leftarrow \leftarrow} = P_{- -} / P_{- \leftarrow}$ . However, due to numerical precision Eq. 5 cannot rank orientation probabilities that are too close to 1 for large  $N$  and iMIIC resorts instead to equivalent v-structure orientation scores,

$$\begin{aligned} \text{score}_v &= -N I'(X; Y; Z | \{A_i\}) + \log 1p(e^{N I'(X; Y; Z | \{A_i\})}) - \log 2 \\ P(x * \rightarrow z) &= P(z \leftarrow * y) = \frac{1}{1 + e^{-\text{score}_v}} \end{aligned} \quad [6]$$

which enable the ordering of orientation probabilities,  $P_1$  and  $P_2$  between alternative v-structures ( $v_1$  and  $v_2$ ), even for very large  $N$ , as  $0 \leq \text{score}_1 < \text{score}_2 < \infty$  is equivalent to  $0.5 \leq P_1 < P_2 < 1$ .

**Induced tail and head orientation scores.** Similarly, induced orientation probabilities originating from an existing arrowhead  $z \leftarrow * y$  can be estimated through the following probability decomposition formula (5),

$$P(x * \bullet z) = P(x * \bullet z | z \leftarrow * y) P(z \leftarrow * y) + P(x * \bullet z | z \rightarrow * y) P(z \rightarrow * y) \quad [7]$$

where  $\bullet$  stands for a tail [resp. a head] depending on the positivity [resp. negativity] of  $I'(X; Y; Z | \{A_i\})$  and a corresponding (conditional) independence  $I'(X; Y | \{A_i\}, Z) \leq 0$  [resp.  $I'(X; Y | \{A_i\}) \leq 0$ ].

However, using the full probability decomposition above can lead to a higher confidence in tail or head induced probabilities than in the head probabilities they derive from, due to the Markov equivalence of non-v-structures. In addition, induced tail / head probabilities become numerically difficult to compare for large  $N$ , as Eq. 7 cannot be expressed in the form of Eq. 6. To circumvent these issues and capture the rationale that the confidence in induced tail / head orientations can only be lower than the confidence in the arrowhead from which they derive, iMIIC redefines the induced tail / head probabilities by retaining only the first term in the probability decomposition above, that is, by assuming that the arrowhead  $z \leftarrow * y$  exists,

$$\begin{aligned} P(x * \bullet z) &= P(x * \bullet z | z \leftarrow * y) P(z \leftarrow * y) \\ &= \frac{1}{1 + e^{-N |I'(X; Y; Z | \{A_i\})|}} \times \frac{1}{1 + e^{-\text{score}_v}} = \frac{1}{1 + e^{-\text{score}_i}} \end{aligned} \quad [8]$$

where we introduced a rectified induced score<sub>i</sub>,

$$\begin{aligned} \text{score}_i &= \max(0, m - \log 1p(e^{-M+m} + e^{-M})) \\ m &= \min(N |I'(X; Y; Z | \{A_i\})|, \text{score}_v) \\ M &= \max(N |I'(X; Y; Z | \{A_i\})|, \text{score}_v) \end{aligned} \quad [9]$$

to enable a global numerical ranking of v-structure orientation and induced orientation probabilities even for very large  $N$  with  $0.5 \leq P_1 < P_2 < 1$  corresponding to  $0 \leq \text{score}_1 < \text{score}_2 < \infty$ .

In addition, when orientation propagation is enforced (*i.e.* step 3 in Fig.1b), an induced tail probability can also be “propagated”, as a head probability, to the other end of the edge, if its end mark is still undefined, *i.e.*,  $P(\underline{x} \leftarrow z) = P(x \circ - z)$ . However, this orientation propagation rule does not rely on specific information in the available data but rather aims at fulfilling the structural assumptions of benchmark graphical models. Hence, propagation has been applied in benchmark comparisons (Fig. 1c,d, Figs. S3-S6) but discarded to analyze real-life data (Figs. 2-5, Figs. S7,S8), in order to ensure that causal discovery on real-life applications is solely based on information actually contained in the available data.

## 5. Orientation confidence and causal nature of edges

Having fully ordered orientation probabilities, even for very large  $N$ , enables to implement edge orientations in decreasing order of confidence rather than any arbitrary order, as implemented in traditional constraint-based methods. In addition, iMIIC allows also to use an orientation confidence threshold  $1 > \beta \geq 0.5$  to enhance the precision of predicted head and tail orientations and, thereby, our confidence in the causal nature of oriented edges. Hence, a genuine causal relation (represented with a green arrow-head) is predicted if the edge can be assigned both significant head and tail probabilities,  $P_h > \beta$  and  $P_t > \beta$ , while a putative causal relation is inferred if only one significant head probability can be assessed given the available observational data, *i.e.*  $P_h > \beta$  and  $P_t \leq \beta$ . Similarly, a bidirected edge, suggesting the effect of an unobserved common cause, is predicted for two significant head probabilities, while all other cases are graphically represented as undirected edges. In practice, orientation precision threshold  $\beta$  mostly impacts the orientations derived from small datasets and has little effects on large datasets such as SEER presented here. All causal discovery benchmark results have also been obtained without enhancing orientation precision (*i.e.* using  $\beta = 0.5$ ) which yields a better balance between precision and recall for all sample size. Finally, iMIIC also allows to include prior knowledge about certain head or tail orientations in graphical models, for instance, to specify contextual variables (*e.g.* sex, year of birth), which cannot be the consequence of other observed or unobserved variables in the dataset, as outlined in the main text.

## 6. Indirect path consistency and information contribution

As mentioned in the overview and limitations, above, traditional constraint-based methods, as well as, the original MIIC method do not control for the global structural consistency of their inferred networks. In particular, there is no guarantee that the separating sets identified during the iterative removal of edges (step 1) remain consistent in terms of indirect paths in the final network. To this end, iMIIC adapts a novel algorithmic scheme (3) to ensure that all separating sets identified to remove dispensable edges are consistent with the final inferred graph. It is achieved by repeating the constraint-based structure learning scheme, iteratively, while searching for separating sets that are consistent with the graph obtained at the previous iteration, as outlined in Fig. 1b. We define two levels of indirect path consistency: skeleton *versus* orientation consistencies. Skeleton consistency guarantees that any node in a separating set is on an indirect path between the extremities of the corresponding removed edge (regardless of orientations along the path), while orientation consistency further enforces that each node in a separating set is a non-descendent neighbor of at least one of these extremities. Importantly, implementing skeleton or orientation consistency of separating sets can be done at a limited complexity cost, through the use of block-cut tree decomposition of graphs (3). All in all, iMIIC indirect path consistency improves the interpretability of the inferred network in terms of indirect effects, which are also quantified with indirect information contributions, based on Eq. 1 including finite size corrections from Eq. 2,

$$\text{IndC}(A_k; XY | \{A_i\}_{k-1}) = \frac{I'(X; Y; A_k | \{A_i\}_{k-1})}{I'(X; Y)} \quad [10]$$

with  $\sum_k \text{IndC}(A_k; XY | \{A_i\}_{k-1}) = 100\% - I'(X; Y | \{A_i\}_n) / I'(X; Y)$ , where  $I'(X; Y | \{A_i\}_n) / I'(X; Y)$  is the residual fraction of mutual information (*i.e.* not accounted for by  $A_1, A_2, \dots, A_n$  indirect contributions given by Eq. 10), which vanishes if the  $XY$  edge has been removed, that is, if  $I'(X; Y | \{A_i\}_n) = 0$ , after negative value rectification.

## References

1. P Spirtes, CN Glymour, R Scheines, D Heckerman, *Causation, prediction, and search*. (MIT press), (2000).
2. J Pearl, *Causality*. (Cambridge university press), (2009).
3. H Li, V Cabeli, N Sella, H Isambert, Constraint-based causal structure learning with consistent separating sets. *Adv. Neural Inf. Process. Syst. (NeurIPS)* **32** (2019).
4. J Zhang, On the completeness of orientation rules for causal discovery in the presence of latent confounders and selection bias. *Artif. Intell.* **172**, 1873–1896 (2008).
5. L Verny, N Sella, S Affeldt, PP Singh, H Isambert, Learning causal networks with latent variables from multivariate information in genomic data. *PLOS Comput. Biol.* **13**, 1–25 (2017).
6. V Cabeli, et al., Learning clinical networks from medical records based on information estimates in mixed-type data. *PLOS Comput. Biol.* **16**, e1007866 (2020).
7. S Affeldt, H Isambert, Robust reconstruction of causal graphical models based on conditional 2-point and 3-point information in *Proceedings of the Thirty-First Conference on Uncertainty in Artificial Intelligence, July 12-16, 2015, Amsterdam, The Netherlands*. (UAI), pp. 42–51 (2015).
8. S Affeldt, L Verny, H Isambert, 3off2: A network reconstruction algorithm based on 2-point and 3-point information statistics. *BMC Bioinforma.* **17**, 12 (2016).

9. TM Cover, JA Thomas, *Elements of Information Theory*. (Wiley), 2nd edition, (2006).
10. V Cabeli, H Li, M da Câmara Ribeiro-Dantas, F Simon, H Isambert, Reliable causal discovery based on mutual information supremum principle for finite datasets in *Paper presented at WHY21 workshop, 35rd Conference on Neural Information Processing Systems*. (NeurIPS), (2021).
11. A Kraskov, H Stögbauer, P Grassberger, Estimating mutual information. *Phys. Rev. E* **69**, 066138 (2004).
12. S Frenzel, B Pompe, Partial mutual information for coupling analysis of multivariate time series. *Phys. Rev. Lett.* **99**, 204101 (2007).
